# Supplementary material for: Multi-Path Bound for DAG Tasks
Source: arXiv:2310.15471 source file (2025-05-14)
Supplement: Supplementary file 1 [file multi_supp.pdf]

# Multi-Path Bound for DAG Tasks: Supplementary Material

Qingqiang He, Nan Guan, Shuai Zhao, and Mingsong Lv

***Abstract*—This is the supplementary material for "Multi-Path Bound for DAG Tasks" [1]. This article provides the full proof for the response time bound derived in [1]. The bound of [1] lifts the constraint that the longest path is required to compute the bound of [2]. The proof in this article generalizes the lemmas and theorems in [2], and most of the text is copied from [2].**

## I. PRELIMINARY

### A. Task Model

A parallel real-time task is modeled as a DAG $G = (V, E)$, where $V$ is the set of vertices and $E \subseteq V \times V$ is the set of edges. Each vertex $v \in V$ represents a piece of sequentially executed workload with worst-case execution time (WCET) $c(v)$. An edge $(v_i, v_j) \in E$ represents the precedence relation between $v_i$ and $v_j$, i.e., $v_j$ can start execution only after vertex $v_i$ finishes its execution. A vertex with no incoming (outgoing) edges is called a *source vertex* (*sink vertex*). Without loss of generality, we assume that $G$ has exactly one source (denoted as $v_{src}$), and one sink (denoted as $v_{snk}$). In case $G$ has multiple source/sink vertices, a dummy source/sink vertex with zero WCET can be added to comply with our assumption.

A *path* is denoted by $\lambda = (\pi_0, \cdots, \pi_k)$, where $\forall i \in [0, k-1] : (\pi_i, \pi_{i+1}) \in E$. We also use $\lambda$ to denote the set of vertices that are in path $\lambda$. The length of a path $\lambda$ is defined as $len(\lambda) := \sum_{\pi_i \in \lambda} c(\pi_i)$. A *complete path* is a path $(\pi_0, \cdots, \pi_k)$ such that $\pi_0 = v_{src}$ and $\pi_k = v_{snk}$, i.e., a complete path is a path starting from the source vertex and ending at the sink vertex. The *longest path* is a complete path with largest $len(\lambda)$ among all paths in $G$, and we use $len(G)$ to denote the length of the longest path. For any vertex set $V' \subset V$, $vol(V') := \sum_{v \in V'} c(v)$. The volume of $G$ is the total workload in the DAG task, defined as $vol(G) := vol(V) = \sum_{v \in V} c(v)$. If there is an edge $(u, v) \in E$, $u$ is a *predecessor* of $v$. If there is a path in $G$ from $u$ to $v$, $u$ is an *ancestor* of $v$. We use $pre(v)$ and $anc(v)$ to denote the set of predecessors and ancestors of $v$, respectively.

**Example 1.** *Fig. 1a shows a DAG task $G$ where the number inside each vertex is its WCET. $v_0$ and $v_5$ are the source and the sink vertex, respectively. The longest path is $\lambda = (v_0, v_1, v_4, v_5)$, so $len(G) = len(\lambda) = 6$. For vertex set $V' = \{v_1, v_3\}$, $vol(V') = 6$. The volume of the DAG $vol(G) = 10$. For vertex $v_4$, $pre(v_4) = \{v_1, v_2\}$, $anc(v_4) = \{v_0, v_1, v_2\}$.*

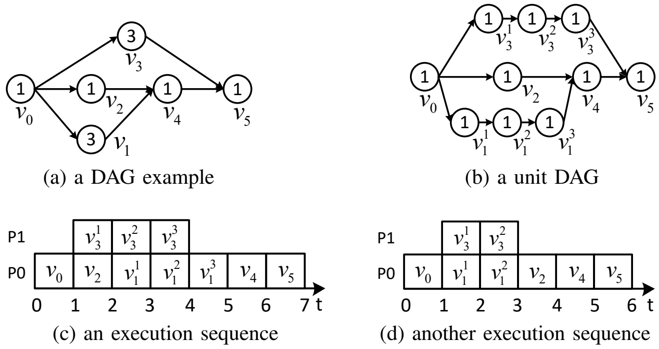

(a) a DAG example
(b) a unit DAG
(c) an execution sequence
(d) another execution sequence

Fig. 1. An illustrative example.

### B. Runtime Behavior

The vertices of DAG task $G$ are scheduled to execute on a multi-core platform with $m$ identical cores $(P_i)_0^{m-1}$ (which is the compact representation of $(P_0, P_1, \cdots, P_{m-1})$ ). A vertex $v$ is *eligible* if all its predecessors have finished execution and thus $v$ can be immediately executed when there are available cores. DAG task $G$ is scheduled by *any* algorithm that satisfies the *work-conserving* property, i.e., an eligible vertex must be executed if there are available cores.

At runtime, vertices of $G$ execute at certain time points on certain cores under the decision of the scheduling algorithm. An *execution sequence* of $G$ describes which vertex executes on which core at every time point.

Since $c(v)$ is the *worst-case* execution time, some vertices may actually execute for less than their WCETs. In an execution sequence $\varepsilon$, a vertex $v$ has an execution time $e(v) \in [0, c(v)]$, which is the accumulated executing time of $v$ in $\varepsilon$. The *start time* $s(v)$ and *finish time* $f(v)$ are the time point when $v$ first starts its execution and completes its execution, respectively. Note that $e(v)$, $s(v)$ and $f(v)$ are all specific to a certain execution sequence $\varepsilon$, but we do not include $\varepsilon$ in their notations for simplicity.

Without loss of generality, we assume the source vertex of $G$ starts execution at time 0, so the *response time* of $G$ in an execution sequence equals $f(v_{snk})$. This paper aims to derive a safe upper bound on the response time $R$ of $G$ in any execution sequence under any work-conserving scheduling.

**Example 2.** *For the DAG $G$ in Fig. 1a, suppose $m = 2$. Two possible execution sequences under work-conserving scheduling*

Qingqiang He is with the School of Computing and Information Technology, Great Bay University, China. E-mail: heqq@gbu.edu.cn.

Nan Guan is with the Department of Computer Science, City University of Hong Kong, China. E-mail: nanguan@cityu.edu.hk.

Shuai Zhao is with the School of Computer Science and Engineering, Sun Yat-sen University, China. E-mail: zhaosh56@mail.sysu.edu.cn.

Mingsong Lv is with the Department of Computing, The Hong Kong Polytechnic University, China. E-mail: mingsong.lyu@polyu.edu.hk.

TABLE I
MAJOR NOTATIONS USED IN THE PAPER

| Notation | Description |
|---|---|
| $\varepsilon$ | an execution sequence |
| $\delta$ | a time unit |
| $c(v)$ | the WCET of vertex $v$ |
| $e(v)$ | the execution time of vertex $v$ |
| $s(v)$ | the start time of vertex $v$ |
| $f(v)$ | the finish time of vertex $v$ |
| $s(\delta)$ | the start time of time unit $\delta$ |
| $f(\delta)$ | the finish time of time unit $\delta$ |
| $len(\lambda)$ | the length of path $\lambda$ |
| $len(G)$ | the length of the longest path of DAG $G$ |
| $vol(V')$ | the volume (total workload) of vertex set $V'$ |
| $vol(G)$ | the volume of $G$ |
| $pre(v)$ | the set of predecessors of vertex $v$ |
| $anc(v)$ | the set of ancestors of vertex $v$ |
| $\lambda^*$ | the critical path (Definition 2) |
| $\lambda^+$ | the restricted critical path (Definition 8) |
| $\omega$ | a virtual path (Definition 4) |
| $len(\omega)$ | the length of virtual path $\omega$ |
| $(\omega_i)_0^k$ | a virtual path list (Definition 5) |
| $(\lambda_i)_0^k$ | a generalized path list (Definition 7) |
| $V'_\varepsilon$ | the projection of $V'$ regarding $\varepsilon$ (Definition 3) |
| $\lambda_\varepsilon$ | the projection of $\lambda$ regarding $\varepsilon$ (Definition 3) |
| $\Delta(V')$ | the workload reduction of $V'$ in $\varepsilon$ (Equation 16) |

*are shown in Fig. 1c and Fig. 1d where $v_1^1$, $v_1^2$ and $v_1^3$ means the execution of first, second and third time unit of $v_1$. In Fig. 1c, every vertex in G executes for its WCET. In Fig. 1d, $v_1$ and $v_3$ execute for less than their WCETs and $e(v_1) = e(v_3) = 2$. In Fig. 1d, the start time and finish time of $v_1$ are $s(v_1) = 1$ and $f(v_1) = 3$, respectively. The response times of G for execution sequences in Fig. 1c and Fig. 1d are 7 and 6, respectively.*

## II. RESPONSE TIME ANALYSIS

This section presents the methodology of deriving a tighter bound for a DAG task. After introducing Lemma 2, an overview of the analysis method is provided in the end of Section II-A. Major notations used in this paper are summarized in Table I.

### A. Analysis on an Execution Sequence

We assume time is discrete and the length of a *time unit* is 1, which is reasonable, because everything in a digital computer is driven by discrete clocks. We use $\delta$ to denote a time unit, and $s(\delta)$ and $f(\delta)$ the start time and finish time of $\delta$.

**Unit DAG.** We transform each vertex of $G$ into a series of *unit vertices*. The WCET $c(v)$ of each unit vertex $v$ is 1 (i.e., a time unit). The resulting DAG is a *unit DAG*. For example, for the DAG in Fig. 1a, the unit DAG is shown in Fig. 1b. Since a time unit cannot be further divided, in an execution sequence, the execution time $e(v)$ of a unit vertex $v$ is either 1 or 0. A unit DAG is also a DAG and notations introduced for DAGs are also applicable to unit DAGs. Unless explicitly specified, $G = (V, E)$ is a unit DAG in Section II. Note that the unit DAG is merely used as an auxiliary concept for the proofs, and our results (i.e., Theorem 1) do *not* need to really transfer the original DAG into a unit DAG.

Our analysis focuses on an *arbitrary* execution sequence $\varepsilon$ of unit DAG $G$. Unless explicitly specified, the following definitions and discussions are all for execution sequence $\varepsilon$.

**Definition 1** (Critical Predecessor [3])**.** *In an execution sequence, vertex $u$ is a* critical predecessor *of vertex $v$, if*

$$u = \arg\max_{u_i \in pre(v)} \{f(u_i)\} \quad (1)$$

**Definition 2** (Critical Path [4])**.** *In an execution sequence, a* critical path $\lambda^* = (\pi_0, \cdots, \pi_k)$ *ending at vertex $v$ is a path satisfying the following two conditions.*

- *$\pi_0 = v_{src} \wedge \pi_k = v$;*
- *$\forall \pi_i \in \lambda^* \setminus \{\pi_0\}$, $\pi_{i-1}$ is a critical predecessor of $\pi_i$.*

As a special case of the above definition, a critical path of $G$ in an execution sequence is a critical path ending at $v_{snk}$. For any vertex $v \neq v_{src}$, since a critical predecessor of $v$ must exist, we can always find the critical path ending at $v$. The critical path is specific to an execution sequence of $G$. A critical path of $G$ in an execution sequence is *not* necessarily the longest path of $G$.

**Example 3.** *For the execution sequence in Fig. 1c, a critical path of G is $(v_0, v_1^1, v_1^2, v_1^3, v_4, v_5)$. In Fig. 1d, a critical path of G is $(v_0, v_2, v_4, v_5)$, which is not the longest path of G.*

**Lemma 1.** *In an execution sequence under work-conserving scheduling on $m$ cores, for any vertex $v$ and its critical predecessor $u$, all $m$ cores are busy in time interval $[f(u), s(v)]$.*

*Proof.* Since $u$ is a critical predecessor of $v$, by Definition 1, $v$ is eligible at $f(u)$. If some core is idle in $[f(u), s(v)]$, it contradicts the fact that the scheduling is work-conserving. □

In an execution sequence, the execution time of some vertices in a vertex set $V'$ may be less than their WCETs. In the following, we introduce notations to describe workloads of vertices in an execution sequence.

**Definition 3** (Projection)**.** *In an execution sequence $\varepsilon$, the* projection *of a vertex set $V'$ is defined as*

$$V'_\varepsilon := \{v \in V' | e(v) = 1 \text{ in } \varepsilon\} \quad (2)$$

*and the projection of a path $\lambda$ is defined as*

$$\lambda_\varepsilon := \{\pi_i \in \lambda | e(\pi_i) = 1 \text{ in } \varepsilon\} \quad (3)$$

Intuitively, a projection $V'_\varepsilon$ is a vertex set including vertices from $V'$ whose execution time is not 0 in $\varepsilon$. As a special case, $V_\varepsilon$ is the projection of the vertex set $V$ of the DAG $G$ in $\varepsilon$. By definition,

$$vol(V'_\varepsilon) = \sum_{v \in V'_\varepsilon} c(v) = \sum_{v \in V'} e(v) \quad (4)$$

$$len(\lambda_\varepsilon) = \sum_{\pi_i \in \lambda_\varepsilon} c(\pi_i) = \sum_{\pi_i \in \lambda} e(\pi_i) \quad (5)$$

**Example 4.** *Consider the execution sequence $\varepsilon$ in Fig. 1d. For vertex set $V' = \{v_1^1, v_1^2, v_1^3, v_3^1, v_3^2, v_3^3\}$, in $\varepsilon$, the execution times of some vertices from $V'$ is 0. $V'_\varepsilon = \{v_1^1, v_1^2, v_3^1, v_3^2\}$. The volume of $V'_\varepsilon$ is $vol(V'_\varepsilon) = 4$, while $vol(V') = 6$. The total workload of G in $\varepsilon$ is $vol(V_\varepsilon) = 8$. For path $\lambda =$*

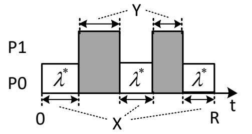


Fig. 2. $X$ and $Y$.

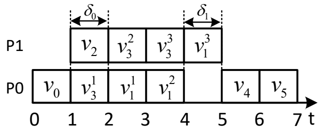


Fig. 3. Workload swapping.

$(v_0, v_1^1, v_1^2, v_1^3, v_4, v_5)$*,* $\lambda_\varepsilon = (v_0, v_1^1, v_1^2, v_4, v_5)$*,* $len(\lambda_\varepsilon) = 5$*, while* $len(\lambda) = 6$*.*

Now we introduce a key concept *virtual path* to describe the *sequentially* executed workload in an execution sequence.

**Definition 4** (Virtual Path)**.** *In an execution sequence, a* virtual path $\omega$ *is a set of vertices executing in different time units.*

Same as path, the length of a virtual path $\omega$ is defined as $len(\omega) := \sum_{v \in \omega} c(v)$. Since virtual path $\omega$ is defined regarding an execution sequence $\varepsilon$, a virtual path does not include vertices whose execution time in $\varepsilon$ is 0. In $\varepsilon$, $\forall v \in \omega$, $e(v) = c(v) = 1$.

All the vertices in a virtual path of $\varepsilon$ do not execute in parallel in $\varepsilon$. In other words, a virtual path is a sequentially executed workload in $\varepsilon$. Note that vertices in a virtual path of $\varepsilon$ may execute in parallel in another execution sequence $\varepsilon'$ of $G$. A path is always a virtual path in any execution sequence. However, a virtual path is not necessarily a path.

**Example 5.** *In Fig. 1c,* $\omega_0 = (v_3^1, v_3^2, v_3^3, v_4)$ *is a virtual path and* $len(\omega_0) = 4$*.* $\omega_0$ *is also a virtual path in the execution sequence in Fig. 1d. In Fig. 1d,* $\omega_1 = (v_1^1, v_3^2, v_2)$ *is a virtual path and* $len(\omega_1) = 3$*.* $\omega_1$ *is not a virtual path in the execution sequence in Fig. 1c, where* $v_1^1$ *and* $v_3^2$ *execute in parallel.*

**Definition 5** (Virtual Path List)**.** *A virtual path list is a set of disjoint virtual paths* $(\omega_i)_0^k$ *(*$k \geq 0$*), i.e.,*

$$\forall i, j \in [0, k],\ \omega_i \cap \omega_j = \varnothing$$

Here $(\omega_i)_0^k$ is the compact representation of $(\omega_0, \cdots, \omega_k)$. Slightly abusing the notation, we also use $(\omega_i)_0^k$ to denote the set of vertices that are in some $\omega_i$ ($i \in [0, k]$).

For critical path $\lambda^*$ of execution sequence $\varepsilon$, we define

- $X$: time interval during which $\exists \pi_i \in \lambda^*$, $\pi_i$ is executing;
- $Y$: time interval before $f(v_{snk})$ during which $\forall \pi_i \in \lambda^*$, $\pi_i$ is *not* executing.

In this paper, a time interval is not necessarily continuous. Fig. 2 illustrates the definitions of $X$ and $Y$. As an example, in Fig. 1d, $X = [0, 1] \cup [3, 6]$, $Y = [1, 3]$, and $|X| = 4$, $|Y| = 2$.

**Workload Swapping.** Next, we introduce a procedure called *workload swapping* which transforms an execution sequence into another one. The purpose of workload swapping is to put the workload into cores in a way that is more convenient to present our analysis. For an execution sequence $\varepsilon$, workload swapping includes the following two operations:

- swap two vertices executing on two cores in the same time unit;
- move a vertex to the same time unit of another idle core (i.e., "swap" a vertex with an "idle block" on another core in the same time unit).

Applying the above procedure to $\varepsilon$ generates a new execution sequence $\varepsilon'$. For a vertex $v$, the core on which $v$ is executing in $\varepsilon$ may be different from that of $\varepsilon'$. Since the start time and finish time of each vertex in $\varepsilon'$ remain the same as $\varepsilon$, the timing behaviors of $\varepsilon$ and $\varepsilon'$ are actually the same. Therefore, the response time $R$ does not change. Time intervals, such as $X$, $Y$, and the critical path do not change either. A virtual path in $\varepsilon$ is still a virtual path in $\varepsilon'$ and virtual path lists do not change. For a path $\lambda$, $\lambda_\varepsilon = \lambda_{\varepsilon'}$.

**Example 6.** *For the execution sequence in Fig. 1c, a new execution sequence generated by workload swapping (swapping* $v_2$ *and* $v_3^1$ *in time unit* $\delta_0$*, and swapping* $v_1^3$ *to core* $P_1$ *in* $\delta_1$*) is shown in Fig. 3.*

**Lemma 2.** $\varepsilon$ *is an execution sequence of DAG* $G$ *under work-conserving scheduling on* $m$ *cores,* $\lambda^*$ *is the critical path of* $\varepsilon$*.* $\lambda^*_\varepsilon$ *is the projection of* $\lambda^*$ *in* $\varepsilon$*. Given a virtual path list* $(\omega_i)_0^k$ *(*$k \in [0, m-1]$*) in* $\varepsilon$ *where* $\omega_0 = \lambda^*_\varepsilon$*, the response time* $R$ *of* $\varepsilon$ *is bounded by:*

$$R \leq len(\lambda^*_\varepsilon) + \frac{vol(V_\varepsilon) - \sum_{i=0}^{k} len(\omega_i)}{m - k} \tag{6}$$

*Proof.* First, we claim the following properties.

A. $R = f(v_{snk}) = |X| + |Y|$ (by definitions of $X$ and $Y$);
B. $|X| = len(\lambda^*_\varepsilon)$ (by the definition of $X$);
C. during time interval $Y$, all cores are busy with vertices from $V_\varepsilon \setminus \lambda^*_\varepsilon$ (by Lemma 1);
D. $(\omega_i)_1^k \subseteq V_\varepsilon \setminus \lambda^*_\varepsilon$ (by Definition 5, virtual paths in a virtual path list are disjoint).

Recall that $vol(V_\varepsilon)$ is the total workload of $G$ in $\varepsilon$. By workload swapping, we swap each virtual path $\omega_i$ to core $P_i$ ($i = 1, ..., k$), which generates a new execution sequence $\varepsilon'$ with the same $X$, $Y$, and $R$ as $\varepsilon$. Let $W$ denote the set of vertices executing in other $m - k$ cores (i.e., $P_0$, $(P_i)_{k+1}^{m-1}$) during $Y$ in $\varepsilon'$, then by Property C, we have

$$|Y| = \frac{vol(W)}{m - k} \tag{7}$$

Since we swap all $(\omega_i)_1^k$ into cores $(P_i)_1^k$, we have

$$W \subseteq I, \text{ where } I := V_\varepsilon \setminus \lambda^*_\varepsilon \setminus (\omega_i)_1^k$$

Therefore, by Property A, B and (7), we have

$$R = |X| + |Y| = len(\lambda^*_\varepsilon) + \frac{vol(W)}{m-k} \leq len(\lambda^*_\varepsilon) + \frac{vol(I)}{m-k} \tag{8}$$

By the definition of $I$ and Property D, we have

$$\begin{aligned} vol(I) &= vol(V_\varepsilon) - len(\lambda^*_\varepsilon) - \sum_{i=1}^{k} len(\omega_i) \\ &= vol(V_\varepsilon) - \sum_{i=0}^{k} len(\omega_i) \end{aligned}$$

which, together with (8), completes the proof. □

**Method Overview.** Lemma 2 gives a response time bound for a particular execution sequence. However, Lemma 2 cannot

be directly used to upper-bound the response time of the DAG as it requires values available only when the execution sequence is given, which is unknown in offline analysis. Therefore, in the following, we will bound these execution-sequence-specific values using static information of the DAG. We rewrite (6) as

$$R \leq len(\lambda_\varepsilon^*) + \frac{vol(V_\varepsilon) - len(\omega_0)}{m-k} - \frac{\sum_{i=1}^{k} len(\omega_i)}{m-k} \quad (9)$$

In Section II-B, we introduce a new abstraction called restricted critical path, and investigate its properties. In Section II-C, using the results of Section II-B, we lower-bound $\sum_{i=1}^{k} len(\omega_i)$ (i.e., lower-bound $\frac{\sum_{i=1}^{k} len(\omega_i)}{m-k}$), and then in Section II-D, we upper-bound $len(\lambda_\varepsilon^*) + \frac{vol(V_\varepsilon) - len(\omega_0)}{m-k}$. Combining them yields an upper bound of the RHS (right-hand side) of (9).

### *B. Restricted Critical Path*

This subsection introduces a key concept *restricted critical path*, which is essentially a critical path identified within a subset of vertices in $G$. In line with the critical path, the restricted critical path is to further characterize the execution behavior of a DAG task with the awareness of multiple long paths in the execution. We first generalize the concept of path.

**Definition 6** (Generalized Path)**.** *A generalized path* $\lambda = (\pi_0, \cdots, \pi_k)$ *is a set of vertices such that* $\forall i \in [0, k-1]$*, there is a path* $\lambda_i$ *starting at* $\pi_i$ *and ending at* $\pi_{i+1}$*. In particular, a vertex set containing only one vertex is a generalized path.*

Intuitively, a generalized path "skips" some vertices in a path so the vertices in a generalized path may not directly connect to each other. For example, in Fig. 1a, $(v_0, v_2, v_4, v_5)$ is a path, while $(v_0, v_2, v_5)$ is a generalized path. Same as path, the length of a generalized path $\lambda$ is defined as $len(\lambda) \coloneqq \sum_{\pi_i \in \lambda} c(\pi_i)$.

The relationship among *path*, *generalized path* and *virtual path* can be summarized as

path $\subseteq$ generalized path $\subseteq$ virtual path

A path must be a generalized path; a generalized path is not necessarily a path. A generalized path must be a virtual path in any execution sequence of $G$; a virtual path in an execution sequence is not necessarily a generalized path. Path and generalized path share a property: vertices in a path or a generalized path always execute sequentially in any execution sequence of $G$. However, this is not true for virtual path: vertices in a virtual path in one execution sequence may not execute sequentially in another execution sequence.

**Definition 7** (Generalized Path List)**.** *A* generalized path list *is a virtual path list, in which each element is a generalized path. A generalized path list is denoted as* $(\lambda_i)_0^k$*, where each* $\lambda_i$ *is a generalized path.*

**Definition 8** (Restricted Critical Path)**.** *For an execution sequence* $\varepsilon$ *and a generalized path list* $(\lambda_i)_0^k$*,* $k \in [0, m-1]$*, the* restricted critical path $\lambda^+ = (\pi_0, \cdots, \pi_j)$ *is a generalized path satisfying (10), (11) and (12):*

$$\pi_j = \underset{u \in (\lambda_i)_0^k}{\arg\max} \{f(u)\} \quad (10)$$

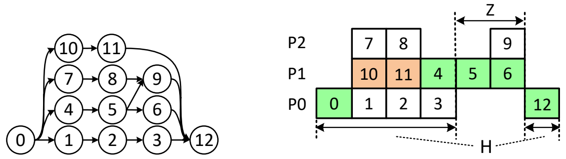


(a) a DAG task (b) an execution sequence

Fig. 4. An example of restricted critical path.

$$\forall \pi_i \in \lambda \setminus \{\pi_0\} : \pi_{i-1} = \underset{u \in anc(\pi_i) \cap (\lambda_i)_0^k}{\arg\max} \{f(u)\} \quad (11)$$

$$anc(\pi_0) \cap (\lambda_i)_0^k = \varnothing \quad (12)$$

Intuitively, the concept of restricted critical path is obtained by applying the concept of critical path to vertices in $(\lambda_i)_0^k$. The restricted critical path ends at the last finishing vertex in $(\lambda_i)_0^k$ (Equation 10). After $\pi_i$ is identified, we identify $\pi_{i-1}$ as the last finishing vertex of ancestors of $\pi_i$ in $(\lambda_i)_0^k$ (Equation 11). This recursive procedure stops until the last identified vertex's ancestor is not in $(\lambda_i)_0^k$ (Equation 12). If $(\lambda_i)_0^k$ includes all vertices of the graph, the restricted critical path of an execution sequence degrades to the critical path of that execution sequence.

**Example 7.** *In Fig. 4a, the number inside vertices is to identify the vertex, not the WCET. The WCET of each vertex is 1. Fig. 4b shows an execution sequence* $\varepsilon$*, and the execution time of each vertex in* $\varepsilon$ *is 1. The number of cores is 3. Let* $\lambda_0 = (v_0, v_1, v_2, v_3, v_{12})$*, which is the longest path. Let* $\lambda_1 = (v_4, v_5, v_6)$*, and* $\lambda_2 = (v_7, v_8, v_9)$*.* $(\lambda)_0^2$ *is a generalized path list. In* $\varepsilon$*, with respect to* $(\lambda)_0^2$*, we can identify a restricted critical path* $\lambda^+ = (v_0, v_4, v_5, v_6, v_{12})$ *(the green vertices).*

Now we transform an execution sequence $\varepsilon$ into a "regular" form by workload swapping.

**Definition 9** (Regular Execution Sequence)**.** *Given an execution sequence* $\varepsilon$ *and a generalized path list* $(\lambda_i)_0^k$ *(*$k \in [0, m-1]$*), we transform* $\varepsilon$ *into a* regular execution sequence $\varepsilon'$ *regarding* $(\lambda_i)_0^k$ *via workload swapping by the following two rules:*

1) *swap* $\lambda_i$ *to core* $P_i$ *for each* $i \in [0, k]$*;*
2) *swap other vertices into cores with a smaller index as much as possible.*

**Lemma 3.** *Let* $v$ *be an arbitrary vertex of* $G$*,* $\delta$ *be a time unit before* $v$ *starts (i.e.,* $f(\delta) \leq s(v)$*) during which some core is idle, then there exists an ancestor of* $v$ *executing in* $\delta$*.*

*Proof.* We prove by contradiction. Assume all ancestors of $v$ do not execute in $\delta$. Let $\lambda^* = (\pi_0, \cdots, \pi_k)$ be the critical path ending at $v$ (i.e., $v = \pi_k$). By our assumption, $\delta$ must be in some time interval when $\lambda^*$ is not executing. By Lemma 1, we know all cores are busy in $\delta$, which contradicts that some cores are idle in $\delta$. The lemma is proved. □

For an execution sequence $\varepsilon$ and a generalized path list $(\lambda_i)_0^k$, $k \in [0, m-1]$, we define

$$v_{fst} = \arg\min_{u \in (\lambda_i)_0^k} \{s(u)\} \quad (13)$$

$$v_{lst} = \arg\max_{u \in (\lambda_i)_0^k} \{f(u)\} \quad (14)$$

Intuitively, for vertices of this generalized path list, $v_{fst}$ is the first vertex to start its execution and $v_{lst}$ is the last vertex to finish its execution in $\varepsilon$. For the restricted critical path $\lambda^+ = (\pi_0, \cdots, \pi_j)$ of $(\lambda_i)_0^k$ in $\varepsilon$, by Definition 8, $f(v_{lst}) = f(\pi_j)$. But generally, $s(v_{fst}) \neq s(\pi_0)$.

**Lemma 4.** *$(\lambda_i)_0^k$, $k \in [0, m-1]$, is a generalized path list. $\varepsilon$ is a regular execution sequence regarding $(\lambda_i)_0^k$. $\lambda^+$ is the restricted critical path of $(\lambda_i)_0^k$ in $\varepsilon$. $\lambda_\varepsilon^+$ is the projection of $\lambda^+$ in $\varepsilon$. There exists a virtual path $\eta$ in $\varepsilon$ satisfying all the following three conditions.*

- (i) $\forall v \in \eta$, $v \notin (\lambda_i)_0^k$;
- (ii) $\forall v \in \eta$, *$v$ executes on* $(P_i)_0^k$;
- (iii) $len(\lambda_\varepsilon^+) + len(\eta) = f(v_{lst}) - s(v_{fst})$.

*Proof.* Let $\lambda^+ = (\pi_0, \cdots, \pi_j)$. By Definition 8 and (13), (14), we have $s(v_{fst}) \leq s(\pi_0)$ and $f(v_{lst}) = f(\pi_j)$. In time interval $[s(v_{fst}), f(v_{lst})]$, either $\lambda^+$ is executing or $\lambda^+$ is not executing. Let $T$ denote the time interval in $[s(v_{fst}), f(v_{lst})]$ during which $\lambda^+$ is not executing. We have

$$len(\lambda_\varepsilon^+) + |T| = f(v_{lst}) - s(v_{fst}) \quad (15)$$

Time interval $T$ can be divided into two disjoint parts: $T_1 := [s(v_{fst}), s(\pi_0)]$ and $T_2 := \bigcup_{h \in [1,j]} [f(\pi_{h-1}), s(\pi_h)]$. Obviously, $T = T_1 \cup T_2$. In the following, we prove that in $[s(v_{fst}), f(v_{lst})]$, whenever $\lambda^+$ is not executing, there is a virtual path $\eta$ that is executing. Specifically, we construct a virtual path $\eta$ by proving that for each time unit $\delta \in T$, there is a vertex $v \notin (\lambda_i)_0^k$ executing on $(P_i)_0^k$ in $\delta$. We prove this by contradiction, assuming that such $v$ does not exist.

In the first step, we focus on time interval $T_2$. For each $h \in [1, j]$, we examine the vertices in each time unit in $[f(\pi_{h-1}), s(\pi_h)]$. There are two cases.

1) In $\delta$, on $(P_i)_0^k$, all $k+1$ vertices are from $(\lambda_i)_0^k$. Suppose that $\pi_h$ executes on core $P_r$ ($r \in [0, k]$) and let $u$ denote the vertex executing on $P_r$ in $\delta$, so $u \in (\lambda_i)_0^k$. Since $u$ executes in $\delta$, we have $f(u) \geq f(\delta)$. Since $\varepsilon$ is a regular execution sequence, if a vertex in $(\lambda_i)_0^k$ executes on $P_r$, this vertex must be in $\lambda_r$, so both $\pi_h$ and $u$ are in $\lambda_r$, which implies that either $\pi_h$ is an ancestor of $u$ or the other way around. Moreover, since $u$ executes in $\delta \in [f(\pi_{h-1}), s(\pi_h)]$, we know $u$ is an ancestor of $\pi_h$. Therefore $\exists u \in anc(\pi_h) \cap (\lambda_i)_0^k$ and $f(u) \geq f(\delta) > f(\pi_{h-1})$.
2) In $\delta$, on $(P_i)_0^k$, less than $k+1$ vertices are from $(\lambda_i)_0^k$. By assumption, all vertices executing in $\delta$ are in $(\lambda_i)_0^k$, thus at least one core is idle in $\delta$. Therefore, by Lemma 3, we know there exists an ancestor of $\pi_h$, denoted by $u$, executing in $\delta$, which implies $f(u) \geq f(\delta)$. By assumption, all vertices executing in $\delta$ are in $(\lambda_i)_0^k$, so $u \in (\lambda_i)_0^k$. Therefore, $\exists u \in anc(\pi_h) \cap (\lambda_i)_0^k$ and $f(u) \geq f(\delta) > f(\pi_{h-1})$.

In summary, for both cases we have proved that $\exists u \in anc(\pi_h) \cap (\lambda_i)_0^k$ and $f(u) > f(\pi_{h-1})$. On the other hand, by Definition 8, in particular (11), $\pi_{h-1}$ has the maximum finish time among vertices in $anc(\pi_h) \cap (\lambda_i)_0^k$, which contradicts the existence of $u$. Therefore, in $T_2$, our assumption must be false, i.e., $\forall h \in [1, j]$, $\forall \delta \in [f(\pi_{h-1}), s(\pi_h)]$, we can find such $v$ satisfying $v \notin (\lambda_i)_0^k$ and $v$ executes on $(P_i)_0^k$ in $\delta$.

In the second step, we focus on time interval $T_1$. By the same reason as $T_2$, we have that $\exists u \in anc(\pi_0) \cap (\lambda_i)_0^k$ and $f(u) > s(v_{fst})$. On the other hand, by Definition 8, in particular (12), there are no ancestors of $\pi_0$ in $(\lambda_i)_0^k$, which contradicts the existence of $u$. Therefore, in $T_1$, our assumption must be false, i.e., $\forall \delta \in [s(v_{fst}), s(\pi_0)]$, we can find such $v$ satisfying $v \notin (\lambda_i)_0^k$ and $v$ executes on $(P_i)_0^k$ in $\delta$.

Summarizing these two steps, we collect such vertices $v$ in each time unit $\delta \in T$. These vertices form a virtual path $\eta$, and $len(\eta) = |T|$. Together with (15), we have $len(\lambda_\varepsilon^+) + len(\eta) = f(v_{lst}) - s(v_{fst})$. The lemma is proved. ☐

**Example 8.** *$(\lambda_i)_0^2$ is the generalized path list in Example 7. Execution sequence $\varepsilon$ in Fig. 4b is a regular execution sequence regarding $(\lambda)_0^2$. In $\varepsilon$, the virtual path $\eta$ identified by Lemma 4 is $\eta = (v_{10}, v_{11})$ (the brown vertices in Fig. 4b).*

By the properties of restricted critical path in Lemma 4, the sequentially executed workload (i.e., the volume of virtual paths) for different complete paths can be analyzed quantitatively in Section II-C.

### C. Lower-bounding $\sum_{i=1}^{k} len(\omega_i)$

This subsection is the most technically challenging part of this work. We develop constructive proofs to derive the desired lower bound. The bound in (6) holds for an arbitrary virtual path list. Therefore, we only need to construct a particular virtual path list for which $\sum_{i=1}^{k} len(\omega_i)$ can be lower-bounded.

In the following, regarding a generalized path list $(\lambda_i)_0^k$, we also use $\lambda$ to denote $\lambda_0$ for conciseness. For an execution sequence $\varepsilon$ and a generalized path list $(\lambda_i)_0^k$, $k \in [0, m-1]$, we define

- $H$: time interval in $[s(v_{fst}), f(v_{lst})]$ during which $\exists \pi_i \in \lambda$, $\pi_i$ is executing;
- $Z$: time interval in $[s(v_{fst}), f(v_{lst})]$ during which $\forall \pi_i \in \lambda$, $\pi_i$ is *not* executing.

By definition, $|H| = len(\lambda_\varepsilon)$, $|H| + |Z| = f(v_{lst}) - s(v_{fst})$. Recall that $\lambda_\varepsilon$ is the projection of $\lambda$ regarding $\varepsilon$ (i.e., eliminating the vertices in $\lambda$ with zero execution time in $\varepsilon$). Note that the definitions of $H$ and $Z$ are different from the definitions of $X$ and $Y$. $X$ is the time interval in which the *critical* path is executing, whereas $H$ is the time interval in which a specific generalized path is executing. As an example, in Fig. 1d, for generalized path list $(\lambda_i)_0^0$ where $\lambda_0 = (v_0, v_1, v_4, v_5)$, $H = [0, 3] \cup [4, 6]$, $Z = [3, 4]$, and $|H| = 5$, $|Z| = 1$.

$H$ and $Z$ are introduced to construct a new virtual path list based on generalized path list $(\lambda_i)_0^k$. Recall the requirements

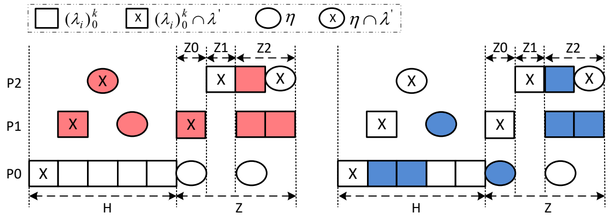


Fig. 5. The construction in Lemma 9. Regular execution sequence $\varepsilon'$ is depicted in the figure. The red vertices represent $W$; the blue vertices represent $W'$. Vertices in $(\lambda_i)_0^k$ are depicted as squares; vertices in $\eta$ as circles. Vertices in $\lambda'$ are labeled with "X". Other vertices are not depicted.

for a virtual path list: 1) vertices in a virtual path must execute sequentially (i.e., execute in different time units); 2) the virtual paths in a virtual path list must be disjoint. These two requirements should be kept in mind when constructing the desired virtual path list.

For a vertex set $V'$ and an execution sequence $\varepsilon$, we define

$$\Delta(V') := vol(V') - vol(V'_\varepsilon) \tag{16}$$

$\Delta(V')$ represents the amount of workload reduction of $V'$ in $\varepsilon$. Obviously, if $V'_0 \subseteq V'_1$, then $\Delta(V'_0) \leq \Delta(V'_1)$. For example, in Fig. 1d, for $V' = \{v_1^1, v_1^2, v_1^3, v_3^1, v_3^2, v_3^3\}$, $\Delta(V') = 6 - 4 = 2$ (see Example 4).

**Lemma 5.** *$W_0$ is a set of vertices. In execution sequence $\varepsilon$, $(\omega_i)_0^k$ is virtual path list satisfying $\bigcup_{i\in[0,k]} \omega_i = W_0$. $\forall v \in W_0$, $\forall u \notin W_0$ satisfying $u$ is in the same time unit as $v$. $W_1 := (W_0 \setminus v) \cup u$. There exists a virtual path list $(\omega'_i)_0^k$ such that $\bigcup_{i\in[0,k]} \omega'_i = W_1$.*

*Proof.* Suppose $v$ is from $\omega_j$. $\omega'_j := (\omega_j \setminus v) \cup u$. Since $v$ and $u$ are in the same time unit, $\omega'_j$ is a virtual path. $\forall i \in [0, k]$, $i \neq j$, $\omega'_i := \omega_i$. Since $u \notin W_0$, obviously, $(\omega'_i)_0^k$ is virtual path list and $\bigcup_{i\in[0,k]} \omega'_i = W_1$. □

Lemma 5 will be used in Lemma 6. Now, we start to construct the desired virtual path list. Again, $\varepsilon$ is an arbitrary execution sequence under analysis. $(\lambda_i)_0^k$ ($k \in [0, m-1]$) is an arbitrary generalized path list. And we also use $\lambda$ to denote $\lambda_0$ for conciseness. For any complete path $\lambda'$ of $G$, we construct a virtual path list $(\omega_i)_0^k$ where $\omega_0 = \lambda'_\varepsilon$. $\lambda'_\varepsilon$ is the projection of $\lambda'$ regarding $\varepsilon$.

After constructing $\omega_0 = \lambda'_\varepsilon$, in the following, we will construct $(\omega_i)_1^k$. The construction of $(\omega_i)_1^k$ will be conducted on two levels. First, we construct a vertex set $W'$ that satisfies $W' = \bigcup_{i\in[1,k]} \omega_i$, i.e., includes all vertices in $(\omega_i)_1^k$. This will be done in Algorithm 1. Second, in Lemma 6, we will prove that we can construct $(\omega_i)_1^k$ using the vertices in $W'$.

We construct $(\omega_i)_1^k$ based on $(\lambda_i)_1^k$. Let $\theta := (\lambda_{i\varepsilon})_1^k \cap \lambda'_\varepsilon$, where $\lambda_{i\varepsilon}$ denotes the projection of $\lambda_i$ regarding $\varepsilon$, i.e., the set of vertices from $\lambda_i$ whose execution time is not 0 in $\varepsilon$ (Definition 3). Since $\lambda'$ is a path, $\theta$ is a generalized path. We transform $\varepsilon$ into a regular execution sequence $\varepsilon'$ regarding $(\lambda_i)_0^k$. Let $\lambda^+$ be the restricted critical path of $(\lambda_i)_0^k$. By Lemma 4, there is a virtual path $\eta$ in $\varepsilon'$ satisfying: (i) $\forall v \in \eta$, $v \notin (\lambda_i)_0^k$; (ii) $\forall v \in \eta$, $v$ executes on $(P_i)_0^k$; (iii) $len(\lambda_\varepsilon^+) + len(\eta) = f(v_{lst}) - s(v_{fst})$. By (i), since $\eta \cap (\lambda_i)_0^k = \varnothing$, $\theta \subseteq (\lambda_i)_0^k$, we have $\eta \cap \theta = \varnothing$. We divide $Z$ into the following time intervals:

- $Z_0$: $\theta$ is executing and $\eta$ is executing;
- $Z_1$: $\theta$ is executing and $\eta$ is not executing;
- $Z_2$: $\theta$ is not executing.

Recall that a time interval is in general not continuous. Obviously, $|Z| = |Z_0| + |Z_1| + |Z_2|$. Let $\eta_H$ denote the set of vertices which is from $\eta$ and is in $H$. Let $\theta_{Z_1}$ denote the set of vertices which is from $\theta$ and is in $Z_1$. We have $len(\theta_{Z_1}) = |Z_1|$. $W := (\lambda_{i\varepsilon})_1^k \cup \eta_H \setminus \theta_{Z_1}$.

Next, based on $W$, we construct a vertex set $W'$ using Algorithm 1. See Fig. 5 for illustration. For time interval $H$, in Line 3-5, we replace all vertices of $\lambda'_\varepsilon$ (squares or circles labeled with "X" in Fig. 5) with vertices of generalized path $\lambda$ (squares in $P_0$). For time interval $Z_0$, in Line 6-8, we replace all vertices of $\lambda'_\varepsilon$ with vertices of $\eta$ (circles). Note that Algorithm 1 is only for the constructive proof, not really needed for computing our new response time bound. We can prove the following properties of $W'$.

**Algorithm 1:** Constructing $W'$

**Input** : $W$, $\lambda'_\varepsilon$
**Output**: $W'$

```
1  W' ← W
2  foreach v ∈ W ∩ λ'_ε do
3      if v is in H then
4          u ← the vertex which is from λ and is in the
           same time unit as v
5          W' ← (W' \ v) ∪ u
6      else if v is in Z_0 then
7          u ← the vertex which is from η and is in the
           same time unit as v
8          W' ← (W' \ v) ∪ u
9      end
10 end
```

**Lemma 6.** *There exists a virtual path list $(\omega_i)_1^k$ satisfying $\bigcup_{i\in[1,k]} \omega_i = W'$.*

*Proof.* By (ii) of Lemma 4, in $\varepsilon'$, $\eta$ executes on $(P_i)_0^k$ and $\eta \cap (\lambda_i)_0^k = \varnothing$. Also in $\varepsilon'$ during $H$, $\lambda_0$ is executing, which means that $\eta_H$ executes on $(P_i)_1^k$. Therefore, In $\varepsilon'$, all vertices of $W$ execute in $(P_i)_1^k$, which means that there exists a virtual path list $(\omega'_i)_1^k$ satisfying $\bigcup_{i\in[1,k]} \omega'_i = W$. By Lemma 5, after each iteration of the loop in Line 2-9 of Algorithm 1, there exists a virtual path list $(\omega_i)_1^k$ satisfying $\bigcup_{i\in[1,k]} \omega_i = W'$. □

**Lemma 7.** $W' \cap \lambda'_\varepsilon = \varnothing$.

*Proof.* In $H$, all vertices from $\lambda'_\varepsilon$ are excluded from $W'$ in Line 3-5 of Algorithm 1. In $Z_0$, all vertices from $\lambda'_\varepsilon$ are excluded from $W'$ in Line 6-8 of Algorithm 1. In $Z_1$, $W \cap \theta_{Z_1} = \varnothing$, which means $W' \cap \theta_{Z_1} = \varnothing$. In $Z_2$, by definition of $Z_2$, $\theta$ is not executing. □

**Lemma 8.** $vol(W') \geq \sum_{i=1}^{k} len(\lambda_i) - \Delta(V) - (len(G) - len(\lambda))$.

*Proof.* By (iii) of Lemma 4,

$$len(\lambda_\varepsilon^+) + len(\eta) = f(v_{lst}) - s(v_{fst})$$

By the definitions of $H$, $Z$,

$$len(\lambda_\varepsilon) + |Z| = f(v_{lst}) - s(v_{fst})$$

We also have $len(G) \geq len(\lambda^+) \geq len(\lambda_\varepsilon^+)$. Therefore,

$$\begin{aligned} len(\eta) - |Z| &= len(\lambda_\varepsilon) - len(\lambda_\varepsilon^+) \\ &= len(\lambda) - \Delta(\lambda) - len(\lambda_\varepsilon^+) \\ &= len(G) - (len(G) - len(\lambda)) - \Delta(\lambda) - len(\lambda_\varepsilon^+) \\ &\geq -\Delta(\lambda) - (len(G) - len(\lambda)) \end{aligned}$$

Let $\eta_{Z_0}$, $\eta_{Z_1}$, $\eta_{Z_2}$ denote the set of vertices which are from $\eta$ and are in $Z_0$, $Z_1$, $Z_2$, respectively. We have $\eta = \eta_H \cup \eta_{Z_0} \cup \eta_{Z_1} \cup \eta_{Z_2}$. By definitions of $Z_0$, $Z_1$, $Z_2$, $len(\eta_{Z_0}) = |Z_0|$, $len(\eta_{Z_1}) = 0$, $len(\eta_{Z_2}) \leq |Z_2|$. We have

$$\begin{aligned} len(\eta_H) &= len(\eta) - len(\eta_{Z_0}) - len(\eta_{Z_1}) - len(\eta_{Z_2}) \\ &\geq len(\eta) - |Z_0| - |Z_2| \end{aligned}$$

Obviously, $len(\theta_{Z_1}) = |Z_1| = |Z| - |Z_0| - |Z_2|$. Therefore,

$$\begin{aligned} len(\eta_H) - len(\theta_{Z_1}) &\geq len(\eta) - |Z| \\ &\geq -\Delta(\lambda) - (len(G) - len(\lambda)) \end{aligned}$$

By (16), $\sum_{i=1}^{k} len(\lambda'_{i\varepsilon}) = \sum_{i=1}^{k} len(\lambda_i) - \Delta((\lambda_i)_1^k)$.

$$\begin{aligned} vol(W') = vol(W) &= \sum_{i=1}^{k} len(\lambda_{i\varepsilon}) + len(\eta_H) - len(\theta_{Z_1}) \\ &= \sum_{i=1}^{k} len(\lambda_i) - \Delta((\lambda_i)_1^k) + len(\eta_H) - len(\theta_{Z_1}) \\ &\geq \sum_{i=1}^{k} len(\lambda_i) - \Delta((\lambda_i)_1^k) - \Delta(\lambda) - (len(G) - len(\lambda)) \\ &= \sum_{i=1}^{k} len(\lambda_i) - \Delta((\lambda_i)_0^k) - (len(G) - len(\lambda)) \\ &\geq \sum_{i=1}^{k} len(\lambda_i) - \Delta(V) - (len(G) - len(\lambda)) \end{aligned}$$

□

**Lemma 9.** *$\varepsilon$ is an execution sequence. $(\lambda_i)_0^k$, $k \in [0, m-1]$, is a generalized path list. Also $\lambda := \lambda_0$. For any complete path $\lambda'$ of $G$, there is a virtual path list $(\omega_i)_0^k$ where $\omega_0 = \lambda'_\varepsilon$, satisfying the following condition.*

$$\sum_{i=1}^{k} len(\omega_i) \geq \sum_{i=1}^{k} len(\lambda_i) - \Delta(V) - (len(G) - len(\lambda)) \quad (17)$$

*Proof.* In the above construction, we have $W'$. By Lemma 6, there exists a virtual path list $(\omega_i)_1^k$ satisfying $\bigcup_{i\in[1,k]} \omega_i = W'$. By Lemma 7, $W' \cap \lambda'_\varepsilon = \varnothing$ which means $(\omega_i)_1^k$ and $\lambda'_\varepsilon$ are disjoint. Therefore, $(\omega_i)_0^k$ where $\omega_0 = \lambda'_\varepsilon$ is a virtual path list. By Lemma 8, we have $\sum_{i=1}^{k} len(\omega_i) = vol(W') \geq \sum_{i=1}^{k} len(\lambda_i) - \Delta(V) - (len(G) - len(\lambda))$. The lemma is proved. □

For Lemma 9, when the first generalized path in $(\lambda_i)_0^k$ is the longest path of $G$, we have $len(\lambda) = len(G)$. Equation (17) degrades to

$$\sum_{i=1}^{k} len(\omega_i) \geq \sum_{i=1}^{k} len(\lambda_i) - \Delta(V) \quad (18)$$

Moreover, when each vertex executes for its WCET in $\varepsilon$, we have $\Delta(V) = 0$. Equation (18) further degrades to

$$\sum_{i=1}^{k} len(\omega_i) \geq \sum_{i=1}^{k} len(\lambda_i) \quad (19)$$

The main idea in the proof of Lemma 9 is to construct $(\omega_i)_1^k$ using $(\lambda_i)_1^k$. $\lambda'_\varepsilon$ is $\omega_0$ and vertices in $(\lambda_i)_1^k \setminus \theta$ are used for $(\omega_i)_1^k$. However, since $\theta$ is in $\lambda'$ and $\lambda'_\varepsilon = \omega_0$, vertices in $\theta$ cannot be used for $(\omega_i)_1^k$ (recall that virtual paths in a virtual path list are disjoint). Therefore, to construct $(\omega_i)_1^k$ using $(\lambda_i)_1^k$ is to replace vertices in $\theta$ using vertices that are not in $\lambda'$. These vertices used to replace $\theta$ are from $\lambda_0$ and $\eta$. We use the following example to explain this.

**Example 9.** *$(\lambda_i)_0^2$ is the generalized path list in Example 7. Let $\lambda' = (v_0, v_4, v_5, v_9, v_{12})$. Since in Fig. 4b each vertex executes for its WCET, $\Delta(V) = 0$. The virtual path $\eta$ identified by Lemma 4 is $\eta = (v_{10}, v_{11})$ (the brown vertices in Fig. 4b). $\theta = (v_4, v_5, v_9)$. $|Z| = |Z_1| = 2$. $v_3$ is to replace $v_4$, and $v_{10}$, $v_{11}$ are to replace $v_5$, $v_9$. Then a new virtual path list $(\omega)_0^2$ is constructed, where $\omega_0 = \lambda'$, $\omega_1 = (v_{10}, v_{11}, v_3, v_6)$, and $\omega_2 = (v_7, v_8)$. We have $vol(\omega_1 \cup \omega_2) = 6 \geq vol(\lambda_1 \cup \lambda_2) = 6$.*

### *D. Bound for the DAG Task*

For concise presentation, we define a function

$$B(x, y, z) := x(1 - \frac{1}{m-k}) + \frac{y - z}{m-k} \quad (20)$$

$B(x, y, z)$ is monotonically increasing with respect to $x$ and $y$, and decreasing with respect to $z$.

Using $B$ function, Lemma 2 can be rewritten as

$$\begin{aligned} R &\leq len(\lambda_\varepsilon^*) + \frac{vol(V_\varepsilon) - \sum_{i=0}^{k} len(\omega_i)}{m-k} \\ &= len(\lambda_\varepsilon^*)(1 - \frac{1}{m-k}) + \frac{vol(V_\varepsilon) - \sum_{i=1}^{k} len(\omega_i)}{m-k} \\ &= B(len(\lambda_\varepsilon^*), vol(V_\varepsilon), \sum_{i=1}^{k} len(\omega_i)) \end{aligned}$$

**Lemma 10.** *Given a generalized path list $(\lambda_i)_0^k$ ($k \in [0, m-1]$), the response time $R$ of DAG $G$ scheduled by work-conserving scheduling on $m$ cores is bounded by:*

$$R \leq len(G) + \frac{vol(G) - \sum_{i=0}^{k} len(\lambda_i)}{m-k} \quad (21)$$

*Proof.* Let $\varepsilon$ be an arbitrary execution sequence of $G$ under work-conserving scheduling. Let $\lambda^*$ denote the critical path of $\varepsilon$. We also use $\lambda$ to denote $\lambda_0$. By Lemma 9, for $\lambda^*$, there is a virtual path list $(\omega_i)_0^k$ where $\omega_0 = \lambda_\varepsilon^*$ satisfying $\sum_{i=1}^k len(\omega_i) \geq \sum_{i=1}^k len(\lambda_i) - \Delta(V) - (len(G) - len(\lambda))$. By Lemma 2, the response time $R$ of $\varepsilon$ satisfies

$$\begin{aligned}
R &\leq B(len(\lambda_\varepsilon^*), vol(V_\varepsilon), \sum_{i=1}^k len(\omega_i)) \\
&\leq B(len(\lambda^*), vol(G) - \Delta(V), \\
&\qquad \sum_{i=1}^k len(\lambda_i) - \Delta(V) - (len(G) - len(\lambda))) \\
&= B(len(\lambda^*), vol(G), \sum_{i=1}^k len(\lambda_i) - (len(G) - len(\lambda))) \\
&= B(len(\lambda^*), vol(G), \sum_{i=0}^k len(\lambda_i) - len(G)) \qquad (22)
\end{aligned}$$

Let $B_0$ denote the bound in (21) and $B_1$ denote the bound in (22).

$$\begin{aligned}
B_0 - B_1 &= len(G) + \frac{vol(G) - \sum_{i=0}^k len(\lambda_i)}{m-k} - \\
&\quad (len(\lambda^*) + \frac{vol(G) - len(\lambda^*) - \sum_{i=0}^k len(\lambda_i) + len(G)}{m-k}) \\
&= len(G) - (len(\lambda^*) + \frac{len(G) - len(\lambda^*)}{m-k}) \\
&= len(G) - len(\lambda^*) - \frac{len(G) - len(\lambda^*)}{m-k} \\
&= (len(G) - len(\lambda^*))(1 - \frac{1}{m-k})
\end{aligned}$$

Since $len(G) \geq len(\lambda^*)$, we have $B_0 - B_1 \geq 0$, which means $B_0 \geq B_1$. The lemma is proved. □

**Theorem 1.** *Given a generalized path list $(\lambda_i)_0^k$ ($k \in [0, m-1]$), the response time $R$ of DAG $G$ scheduled by work-conserving scheduling on $m$ cores is bounded by:*

$$R \leq \min_{j \in [0,k]} \left\{ len(G) + \frac{vol(G) - \sum_{i=0}^j len(\lambda_i)}{m-j} \right\} \qquad (23)$$

*Proof.* By Lemma 10, we know that for each $j \in [0, k]$, $len(G) + \frac{vol(G) - \sum_{i=0}^j len(\lambda_i)}{m-j}$ is an upper bound of $R$. Therefore, the minimum of these bounds also upper-bounds $R$. □

The derivation procedure of the bound in Theorem 1 is based on unit DAGs. However, the result of Theorem 1 can be directly applied to the original DAG. For a DAG $G$ and its corresponding unit DAG $G^u$, $vol(G) = vol(G^u)$; for a path $\lambda$ of $G$, and its corresponding path $\lambda^u$ of $G^u$, $len(\lambda) = len(\lambda^u)$. For example, in Fig. 1a, let $\lambda = (v_0, v_1)$; in Fig. 1b, the corresponding path is $\lambda^u = (v_0, v_1^1, v_1^2, v_1^3)$. Obviously, $len(\lambda) = len(\lambda^u) = 4$. Therefore, the result of Theorem 1 directly applies to the original DAG $G$.

Note that by our analysis, the bound in (23) is still safe when some vertices execute for less than their WCETs. The derivation of our bound only depends on the work-conserving property. Same as Graham's bound [5], our bound is valid for any work-conserving scheduling algorithm, regardless of whether it is preemptive or non-preemptive, priority-based or other rule-based.

## References


[1] Q. He, N. Guan, S. Zhao, and M. Lv, "Multi-path bound for DAG tasks," *IEEE Transactions on Computer-Aided Design of Integrated Circuits and Systems*, 2024.

[2] Q. He, N. Guan, M. Lv, X. Jiang, and W. Chang, "Bounding the response time of DAG tasks using long paths," in *2022 IEEE Real-Time Systems Symposium (RTSS)*. IEEE, 2022, pp. 474–486.

[3] J. Sun, F. Li, N. Guan, W. Zhu, M. Xiang, Z. Guo, and W. Yi, "On computing exact wcrt for dag tasks," in *2020 57th ACM/IEEE Design Automation Conference (DAC)*. IEEE, 2020, pp. 1–6.

[4] Q. He, X. Jiang, N. Guan, and Z. Guo, "Intra-task priority assignment in real-time scheduling of dag tasks on multi-cores," *IEEE Transactions on Parallel and Distributed Systems*, vol. 30, no. 10, pp. 2283–2295, 2019.

[5] R. L. Graham, "Bounds on multiprocessing timing anomalies," *SIAM journal on Applied Mathematics*, vol. 17, no. 2, pp. 416–429, 1969.
